# Supplementary material for: Entropy in the non-Fermi-liquid regime of the doped $2d$ Hubbard model
Source: arXiv:2001.09948 ancillary file (2020-12-23)
Supplement: Supplementary file 1 [file SM.pdf]

# Supplemental Material for "Entropy in the non-Fermi-liquid regime of the doped 2d Hubbard model"


Connor Lenihan,[1] Aaram J. Kim,[1] Fedor Šimkovic IV.,[1,2,3] and Evgeny Kozik[1]

[1] *Department of Physics, King's College London, Strand, London WC2R 2LS, UK*
[2] *Centre de Physique Théorique, École Polytechnique, CNRS, Université Paris-Saclay, 91128 Palaiseau, France*
[3] *Collège de France, 11 place Marcelin Berthelot, 75005 Paris, France*


The thermodynamic quantities in Eq. (2) of the main text were obtained by the diagrammatic Monte Carlo method, where an intensive observable $A$ is represented by the sum of all connected Feynman diagrams corresponding to its Taylor-series expansion in the powers of the bare coupling $U$,

$$A = \sum_m a_m U^m, \tag{1}$$

directly in the thermodynamic limit (TDL). The specific expansion is constructed using the non-interacting Green's function $G_0$ with a shifted by $n_0 U$ chemical potential [1, 2], $\mu \to \mu - n_0 U$, where $n_0$ is the non-interacting density per spin component determined self-consistently by $G_0$. The shift improves the convergence properties of the diagrammatic series relative to the original expansion [3] but also reduces the Monte Carlo variance [4] in the CDet algorithm [5] used for sampling the series. CDet enables efficient summation of the connected diagrams directly in the TDL by expressing the sum over all diagram topologies for a given vertex configuration by means of the determinant of a matrix built on the propagators $G_0$ connecting the vertices [1, 2], and recursively subtracting the disconnected contributions. The summation/integration over the vertex positions is then performed by Monte Carlo sampling.

The algorithm allows us to compute the coefficients $a_m$ numerically exactly with sufficiently small error bars up to the maximum truncation order $m_* \sim 10$. To reconstruct the observable from its series (1) in the correlated regime given a finite number of coefficients, we follow the protocol of Ref. [4]. Convergence of the series is controlled by the location of the singularity $U_s$ closest to the origin in the complex plane $U$. The locations of the singularities can be found by the D-log Padé method [6–8], which also allows us to reconstruct the value of the observable from its Taylor-series expansion. The systematic error of the D-log Padé extrapolation is found as the discrepancy between the results obtained for different free parameters of the scheme, given the statistical error bars, as demonstrated in Ref. [4].

Generically, the singularities in the complex plane of $U$ do not preclude controlled evaluation of the observable even if the series turns out to be divergent as a result. However, reconstructing the observable breaks down when a singularity appears exactly on the real axis

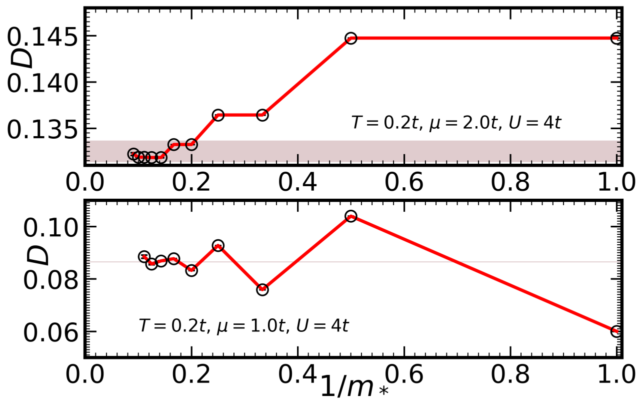


Figure 1: Double occupancy as a function of inverse truncation order $m_*$ at $T = 0.2t$, $U = 4t$ for $\mu = 2.0$ ($n = 1$, top panel) and $\mu = 1.0$ ($n = 0.8381(4)$, bottom panel). The horizontal red bars represent the error bounds on the extrapolation to infinite order using the D-log Padé technique, which include both the statistical and systematic error.

with $0 < U_s < U$. This may happen when the system experiences a second-order phase transition at $U_s$ and therefore the phase at $U > U_s$ can not be described in terms of the normal-state diagrammatics. A phase transition is not expected at half-filling due to the Mermin-Wagner theorem, but also in the doped case at our temperatures of interest. Nonetheless, since the coefficients $a_m$ have error bars, we are often unable to resolve the singularity with a purely real $U_s$ from a pair of complex-conjugate singularities close to the real axis. Such a situation occurs at half-filling when the antiferromagnetic (AFM) correlation length extends beyond $\sim 10$ lattice sites [9]. It is natural that the long correlation length is reflected in the singularity structure of local observables in a way very similar to a true phase transition, resolving the difference requiring the knowledge of the series coefficients $a_m$ with sufficiently small error bars up to a sufficiently high order. Thus, with the accuracy and number of the coefficients at hand, the reliability of our method is limited by how close this pair of singularities, which appear as a single singularity on the real axis, is to the value of the interaction $U$ that we are interested in.

It is tempting to regularize the series by limiting the system size to a finite value, which cuts off the correlation length and pushes the singularities away from the real axis accordingly. The tradeoff, however, is that the observable acquires a substantial system-size dependence, extrapolating which to the TDL could be very challenging [10]. We therefore keep the system size infinite in all our calculations.

Figure 1 illustrates the evaluation of thermodynamic observables by the example of double occupancy $D$ at two different densities, $n = 1$ ($\mu = 2.0t$, half-filling) and $n = 0.8381(4)$ ($\mu = 1.0t$), at $T = 0.2t$ and $U = 4t$. It shows partial sums for $D$ against the inverse truncation order and the result of the extrapolation by the D-log Padé method, which includes both the statistical and systematic error of extrapolation [4]. At half-filling, the pair of singularities due to the AFM crossover [9] appears as a single singularity at $U_s = 5.3(5)t$. Since the singularity is close to $U = 4t$ we are interested in, the convergence of the series is slow and the extrapolated value has a substantial error bar. This singularity is the reason why the maximum $U$ value for which the results are analyzed in this work is limited to $4t$. However, as the system is doped, the apparent AFM singularity moves farther away from the origin, reaching $U_s \approx 9t$ for $n = 0.8381(4)$ at ($\mu = 1.0t$), consistent with weakening AFM correlations. Other singularities in the negative half-plane, namely at $U_s \approx -4 \pm i$ control the convergence in this case and lead to the more pronounced oscillations with diagram order. They are, however, not restricting the accuracy of the extrapolation because they are a large distance away from the physical value $U = 4t$. This explains the drastic difference between the error bars in the two example cases and the reduction of the errors with doping for all data in the main text. In fact, at $\mu = 1.0t$, the apparent singularity at $U_s \approx 9t$ allows us to obtain accurate results at much larger $U \sim 7t$, but we limit the scope to $U = 4t$ because the crossover physics is essentially due to the extending AFM correlations near half-filling.

Figure 2 compares the entropy obtained in this work in the TDL with the results on the $4\times4$ lattice by the Finite Temperature Lanczos Method (FTLM) [14] for $T = 0.2$ and $T = 0.3$ and the well established methods at half filling: the extrapolated to the TDL Dynamical Cluster Approximation (DCA) [11], Variational Cluster Approximation (VCA) and Numerical Linked Cluster Expansions (NLCE) [13]. The DCA data at $T = 0.2$, and the NLCE data at $T = 0.3$ are in perfect agreement with our results, while the DCA result at $T = 0.3$ is consistent, being only within two error bars. The data for $s(\mu)$ in Fig. 2(b) for the FTLM is obtained by using $n(\mu)$ in the TDL from our own calculations. Close to half-filling the FTLM predicts a significantly smaller entropy and, as a consequence, a dramatically smaller range of the non-Fermi liquid (NFL) regime. At the lower temperature of $T = 0.2$ the $\sim 25\%$ lower entropy for small doping leads

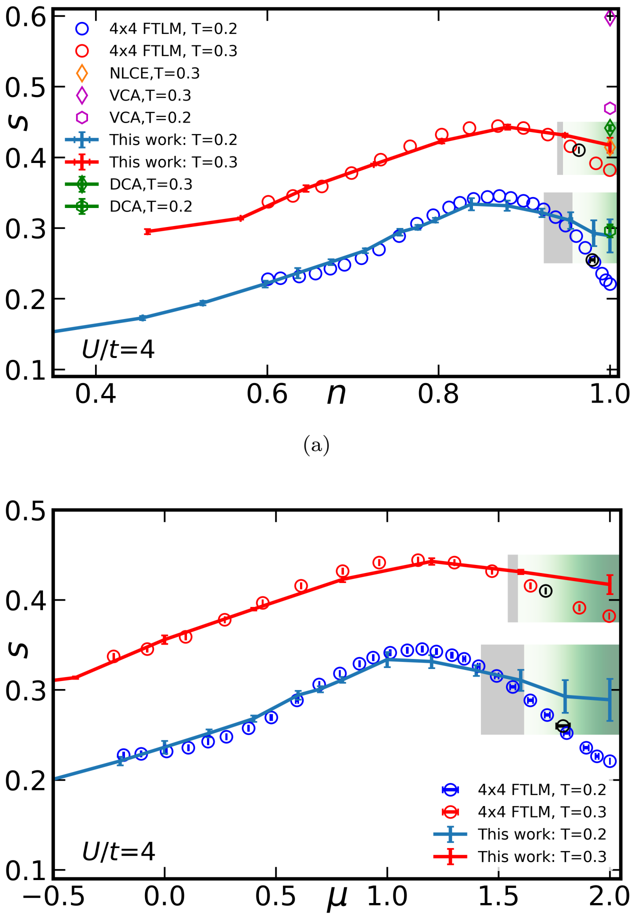


(a)

(b)

Figure 2: Comparison of the entropy obtained in this work in the TDL with that found by other methods at $U = 4t$ and two temperatures $T = 0.2t$ and $T = 0.3t$. The black points represent the crossover to the NFL regime for the FTLM data on a $4 \times 4$ lattice and the gray bars the same for our data. The green shading hence represents the extent of the NFL regime. Panel (a) shows entropy as a function of density and includes a comparison to the results obtained at half-filling by DCA [11], VCA [12] and NLCE [13]. Panel (b) shows the corresponding entropy against $\mu$ from which the NFL crossover can be pinpointed as the inflection point; the dependence of the FTLM data on $\mu$ is obtained using our controlled data for $n(\mu)$ in the TDL.

to the inflection point—represented by the gray bar for our data and by black points for the FTLM—appearing at only $\sim 3\%$ doping which would lead to the mistaken conclusion that the $U = 4t$, $T = 0.2t$ Hubbard model has a very narrow range for the NFL and hence is weakly correlated and irrelevant for the problem of high-$T_c$ superconductivity. Since the FTLM is essentially exact for the finite-size system, we can conclude that the discrepancy between the methods can be attributed to long-range cor-

relations persisting with doping into the NFL regime. In consistency with this interpretation, the discrepancy between the finite-size and the TDL data becomes smaller at the higher $T = 0.3t$.


[1] A. Rubtsov, arXiv:cond-mat/0302228. (2003).

[2] A. N. Rubtsov, V. V. Savkin, and A. I. Lichtenstein, Phys. Rev. B **72**, 035122 (2005).

[3] W. Wu, M. Ferrero, A. Georges, and E. Kozik, Phys. Rev. B **96**, 041105 (2017).

[4] F. Šimkovic and E. Kozik, Physical Review B **100** (2019).

[5] R. Rossi, Phys. Rev. Lett. **119**, 045701 (2017).

[6] G. A. Baker Jr, Physical Review **124**, 768 (1961).

[7] D. L. Hunter and G. A. Baker, Phys. Rev. B **7**, 3346 (1973).

[8] G. A. Baker Jr, *Essentials of Padé Approximants* (Academic Press, 1975).

[9] A. J. Kim, F. Simkovic, and E. Kozik, Phys. Rev. Lett. **124**, 117602 (2020).

[10] F. Šimkovic, J. P. F. LeBlanc, A. J. Kim, Y. Deng, N. V. Prokof'ev, B. V. Svistunov, and E. Kozik, Phys. Rev. Lett. **124**, 017003 (2020).

[11] J. P. F. LeBlanc and E. Gull, Phys. Rev. B **88**, 155108 (2013).

[12] K. Seki, T. Shirakawa, and S. Yunoki, Physical Review B **98** (2018), 10.1103/physrevb.98.205114.

[13] E. Khatami and M. Rigol, Phys. Rev. A **84**, 053611 (2011).

[14] J. Bonča and P. Prelovšek, Phys. Rev. B **67**, 085103 (2003).
